# Supplementary material for: OLALA: Object-Level Active Learning for Efficient Document Layout Annotation
Source: arXiv:2010.01762 source file (2021-03-29)
Supplement: Supplementary file 1 [file notation.tex]

\begin{table}[h]
    \centering
    \resizebox{1.\linewidth}{!}{
    \begin{threeparttable}
        \begin{tabular}{cl}
        \toprule
        Notation      & Meaning \\ 
        \midrule
        $\bar{Y}_i$   & Manually created object labels for $i$-th input \\
        $\hat{Y}_i$   & Model predicted object labels for $i$-th input  \\
        $\tilde{Y}_i$ & Combined object annotations for $i$-th input \\
        \midrule
        $t$           & Number of labeling rounds \\
        $r$           & Object selection ratio during AL \\
        $m$           & Labeling budget (number of objects to label) \\
        $\xi$         & IOU threshold in Duplication Removal \\
        $\alpha$      & \multirow{2}{*}{The horizontal and vertical object shift ratio} \\
        $\beta$       \\
        \bottomrule
        \end{tabular}
    \end{threeparttable}
    }
\caption{Notations and their meanings in \Olala}
\label{table:notation}
\end{table}
